# Supplementary material for: Response properties in phaseless auxiliary field quantum Monte Carlo
Source: arXiv:2308.05530 source file (2023-08-10)
Supplement: Supplementary file 1 [file si.pdf]

# Supporting information

## Convergence of backpropagation AFQMC estimators

The following figures show the convergence of dipole moments for BP-AFQMC calculations with back-propagation time ( $\tau_{BP}$ ) reported in Table I of the main text. These calculations were performed with QMCPACK using 6000 blocks of 50 steps each, with a time step of 0.01 a.u.

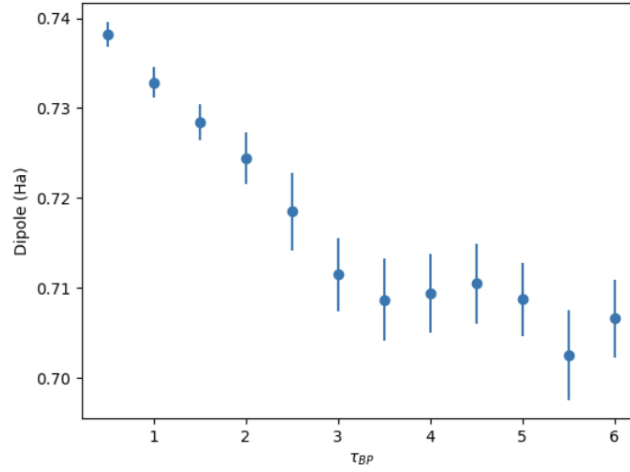

Figure 1: H<sub>2</sub>O

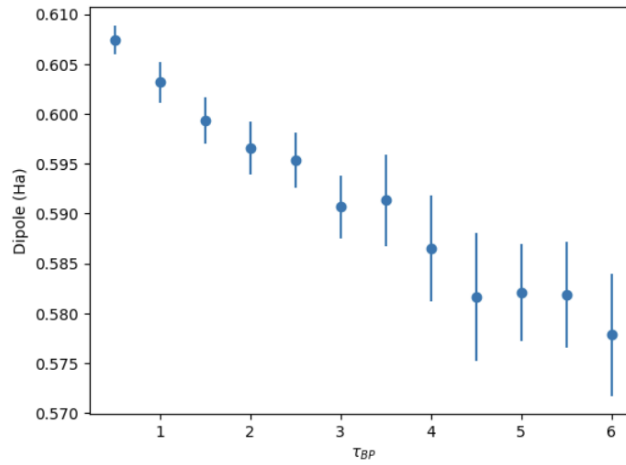

Figure 2: NH<sub>3</sub>

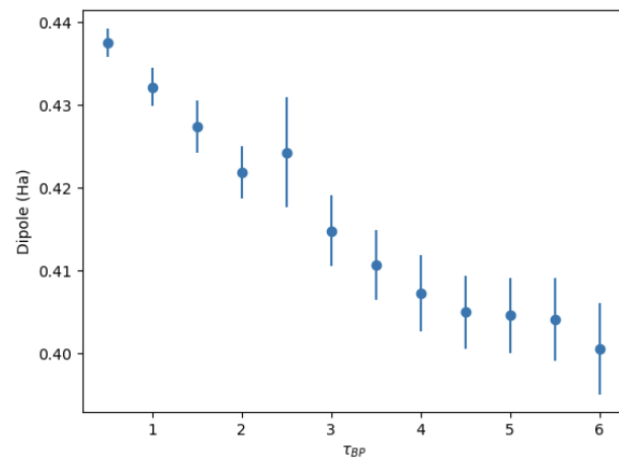

Figure 3: HCl

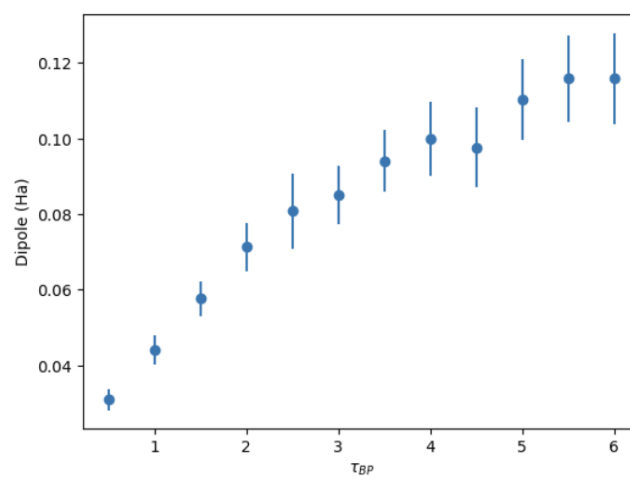

Figure 4: CO

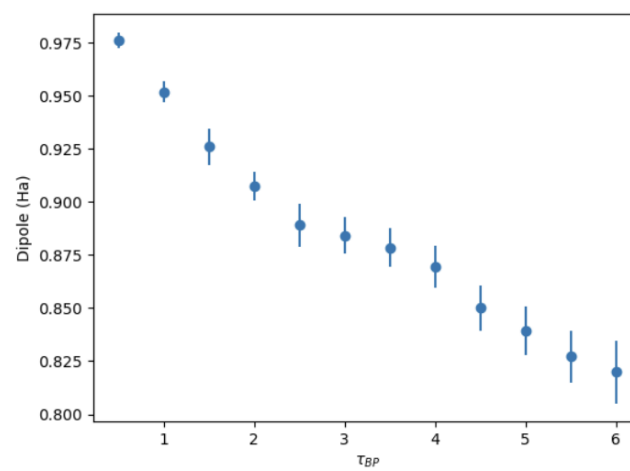

Figure 5: CH<sub>2</sub>O
